# Supplementary material for: Improving Data-Efficient Fossil Segmentation via Model Editing
Source: arXiv:2210.03879 source file (2023-04-10)
Supplement: Supplementary file 9 [file wacv2023_reviews.pdf]

# View Reviews

## Paper ID

79

## Paper Title

Improving Fine-Grain Segmentation via Interpretable Modifications: A Case Study in Fossil Segmentation

## Track Name

Round 1

## Reviewer #1

---

### Questions

#### 1. Paper Summary

The paper discusses how different interpretability techniques (such as perturbation, inpainting and texture synthesis) can be used to improve segmentation of fine-grained objects in absence of a huge labeled dataset. Specifically, the paper focuses on Fossil Segmentation, an area that demands domain-expert knowledge to annotate data, thus, making the annotation process very time consuming. In this paper, techniques like image perturbation are used to identify the limitations of the segmentation model (in this case, Mask-RCNN) and then a model editing technique is applied to rectify the identified mistakes. Findings of the paper are showcased on a small dataset containing only 10 images.

#### 2. Strengths

- The concept is straight-forward and easy to understand.
- Clearly explained the weaknesses of the Mask-RCNN model for the task at hand.
- The main novelty of the paper is in its approach for mitigating the model weaknesses. Specifically, the paper extended an existing model editing technique from image classification to image segmentation. The paper super-categorizes multiple background classes into a single background class from which the target class can be easily distinguished.

#### 3. Weaknesses

- The organization of the paper can be improved. For example, in Lines 250-258, the paper discusses that their modified Mask R-CNN do not work well. The explanation of why it doesn't perform well is not properly explained. Moreover, they pose this as a motivation for analyzing and addressing the failures of the model. This seemed to me a bit abrupt. If this is the main motivation, they should mention it earlier in the paper, preferably in the introduction, and not in the related work section.
- Novelty is limited. Research contribution is also minimal. Some of the concepts (like, image occlusion, synthetic texture, etc.) might be novel for the fossil segmentation domain; but for general deep learning/computer vision community, these are extensively used approaches. The reviewer did not find any novelties on developing new techniques for the computer vision area in general.
- The main concern for this reviewer arises from the limited experimental set-up. The training data is extremely small and thus, the conclusion drawn from such a small dataset is not very convincing.
- The topic is restricted to one specific use case. This might not be interesting to a broader audience that is usually addressed in a WACV conference.
- The paper mentions that the proposed paradigm can be applied to other segmentation models, but they have not shown any experiment to support this claim.

#### 4. Recommendation

Weak Reject

## 5. Justification

Some other concerns are -

1. No details about the dataset (except the number of images) is provided.
2. The paper mentions having different rock samples of varied appearance (lines 145-147). Experiments on different rock samples would have been better to understand the strengths and weaknesses of the method.
3. Why are the experiments only based on the MASK-RCNN model? Do other SOTA segmentation models also fail for the fossil segmentation task? Comparing the performance of different segmentation models (SOTA ones) would have been helpful to understand the importance of the paradigm proposed in this paper.
4. The paper talks about exclusive training, validation and test subsets. However, the results are shown by combining the validation and test images. Usually, in deep learning community, the validation results are somewhat biased as we tune our training model based on the validation dataset.

Please refer to the weaknesses for further details.

## Reviewer #2

---

## Questions

### 1. Paper Summary

The authors focuses on the fine-grained segmentation considering Fossils domain in which very small objects are present such as Archaeocyathid and Calcimicrobes. Due to the absence of labeled datasets with semantic segmentation masks they tried to improve a Mask-RCNN model using model-editing techniques for correcting systematic classification mistakes.

### 2. Strengths

The authors proposed to solve a very hard semantic segmentation task considering the fossils domains in which small objects are present. This kind of objects have irregular shapes and sizes and they are present on rocks. The authors identify weakness of standard segmentation models like Mask-RCNN considering this constrained domain. They propose an approach that with the use of model-editing technique improves the performance using only few images.

### 3. Weaknesses

The authors claimed the absence of datasets labeled with semantic masks considering the fossils domain. They used a very small dataset composed of 10 images. It is not clear how these images have been acquired and annotated and if the authors would release this dataset for research purposes. I think that the dimension of the dataset is a very weak point of this work even they are considering the problem of semantic segmentation using few images. The authors should justify this choice and give strong motivation for this. Moreover, the experiments are very confused, all the performance seems to be similar (e.g., the difference is only about few points). Consider this, what is the real contribute of this study? Why researchers should follow the author's approach? The performed experiments are solid considering only a dataset of 10 images? I think that in a real scenario, this method can not be useful to solve a real problem.

Another weak point is related to the order of tables and images, during the read of the paper table/images are referenced without a specific order and this confuses readers. Please, I suggest to improve the quality of the structure of the paper adjusting the order of tables and images.

### 4. Recommendation

Borderline (Revise and Resubmit)

### 5. Justification

Considering my comments I suggest the authors to improve this work. At the actual stage this work is not ready to be published in this conference.

## Questions

### 1. Paper Summary

The paper presents an application of the paper[1] for the segmentation of ancient reef fossils in rock samples. Unlike the COCO dataset, the annotation for these reef fossil images requires both domain expertise and longer time durations, which forces the authors to work with a very small set of images. The authors first identify the weakness in Mask R-CNN to identify the different fossil classes and then try to address the shortcomings of Mask R-CNN taking inspiration from [1] by using the newly collected small dataset. They report the precision, recall, and intersection over union(IoU) on the dataset for the new dataset.

### 2. Strengths

1. The paper is well written and easy to follow and the authors do a good job to show why their work matters and how can it be beneficial.
2. The authors have shown why Mask R-CNN can not be used directly for such fine-grained segmentation works and why they resolve to use the model-editing[1] process.
- 3, The results show an improved precision when editing the model using a single image.
4. The authors do a comprehensive evaluation to show scenarios for both types of archaeocyathids. The model performance differs between the two archaeocyathids types due to their different appearance.

[1]: Shibani Santurkar, Dimitris Tsipras, Mahalaxmi Elango, David Bau, Antonio Torralba, and Aleksander Madry. Editing a classifier by rewriting its prediction rules. In NeurIPS, 2021.

### 3. Weaknesses

1. The authors show multiple evaluations of their model with an increase in precision, however, this often leads to a decrease in recall. I would recommend reporting the F1 score also.
2. The model editing method changes the weights in order to map certain concepts(keys) to certain other concepts(values). Since the authors deal with binary segmentation, all the non-archaeocyathids are mapped to red mud. So the order of images should not matter but the different results show that order affects the results. Can the authors comment on this as to why they think the order matters while training?
3. In Table 7, are the results are shown for unperturbed test images or perturbed test images?

### 4. Recommendation

Weak Accept

### 5. Justification

The paper presents a good use case of [1] for segmenting ancient reefs. Identifying and segmenting images of these reefs is a laborious task and automating this process can save a lot of time. This work can be further developed which can results in a good application. While there is a lot of scope in the direction this work progresses, however, the improvement seems minor. The gain in precision is marked by a decreasing recall and IoU. Still, the work explores different cases and the evaluation provided is comprehensive which is why I am leaning towards weak acceptance, however, I would be happy to change my decision based on the author's replies.

[1] Shibani Santurkar, Dimitris Tsipras, Mahalaxmi Elango, David Bau, Antonio Torralba, and Aleksander Madry. Editing a classifier by rewriting its prediction rules. In NeurIPS, 2021.
